# Supplementary material for: Intrinsic and extrinsic plasmons in the hard x-ray photoelectron spectra of nearly free electron metals
Source: arXiv:2404.16620 source file (2024-04-25)
Supplement: Supplementary file 1 [file AlMgPlasmon_haxpes_SM_arxiv.pdf]

# Supplementary material for "Intrinsic and extrinsic plasmons in the hard x-ray photoelectron spectra of nearly free electron metals"

Mohammad Balal[1], Shuvam Sarkar[1], Pramod Bhakuni[1],
Andrei Gloskovskii[2], Aparna Chakrabarti[3,4], Sudipta Roy Barman[1]

[1]*UGC-DAE Consortium for Scientific Research,*
*Khandwa Road, Indore 452001, India*

[2]*Deutsches Elektronen-Synchrotron DESY,*
*Notkestrasse 85, D-22607 Hamburg, Germany*

[4]*Raja Ramanna Centre for Advanced Technology,*
*Indore 452013, Madhya Pradesh, India and*

[3]*Homi Bhabha National Institute, Training School Complex,*
*Anushakti Nagar, Mumbai 400094, Maharashtra, India*

**The Supplementary material contains six figures (Figs. S1-S6).**

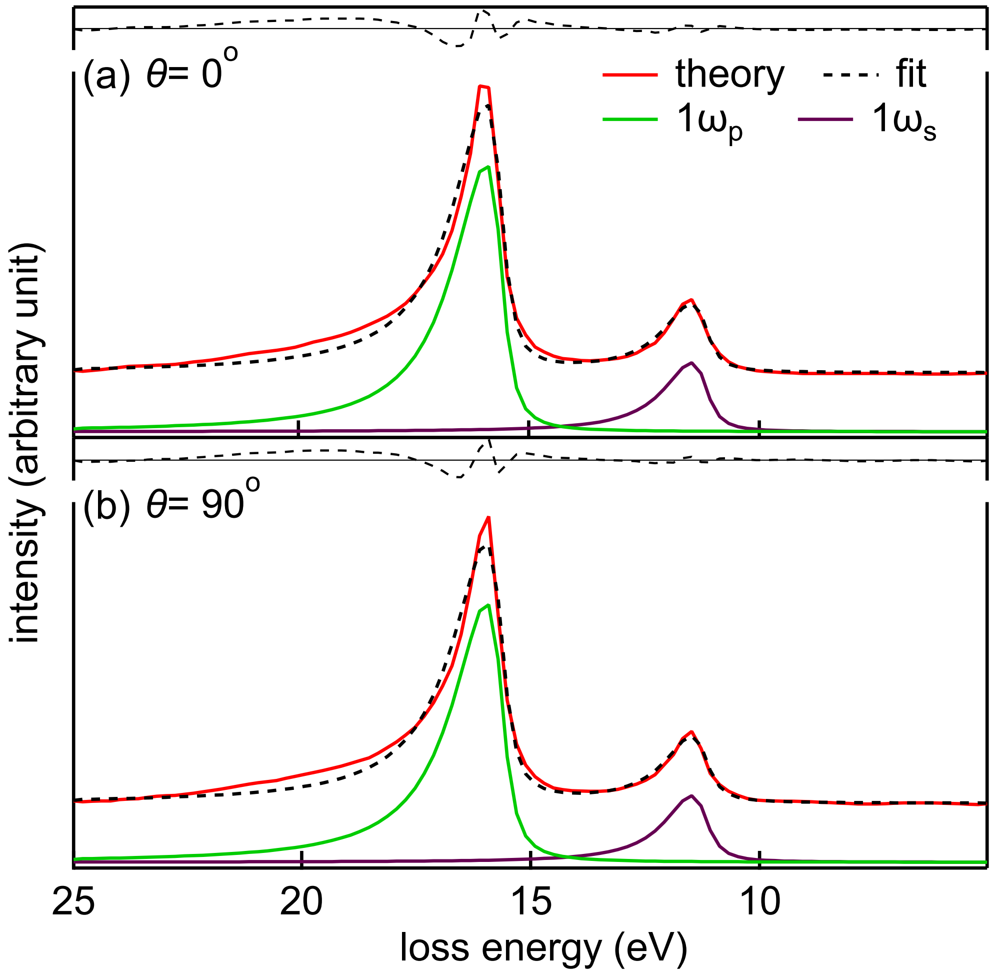


FIG. S 1. The theoretical $1\omega_p$ and $1\omega_s$ line shapes (red curve) from Figs. 2(c) and 3 of Ref. 1 calculated for $h\nu$= 5 keV at (a) grazing emission ($\theta$= 0°) and (b) normal ($\theta$= 90°) have been fitted with two asymmetric Lorentzians representing the $1\omega_s$ (violet) and $1\omega_p$ (green) plasmons. The fitted curve is shown as black dashed curve, and the residual is shown in the top panel.

[1] H. Shinotsuka, T. Uwatoko, T. Konishi, and T. Fujikawa, J. Surf. Anal. **14**, 332 (2008).

[2] D. R. Penn, Phys. Rev. Lett. **40**, 568 (1978).

[3] H. Höechst, P. Steiner, and S. Hüfner, Z. Physik B **30**, 145 (1978).

[4] P. Leonard J. Phys. F: Met. Phys. **8**, 467 (1978).

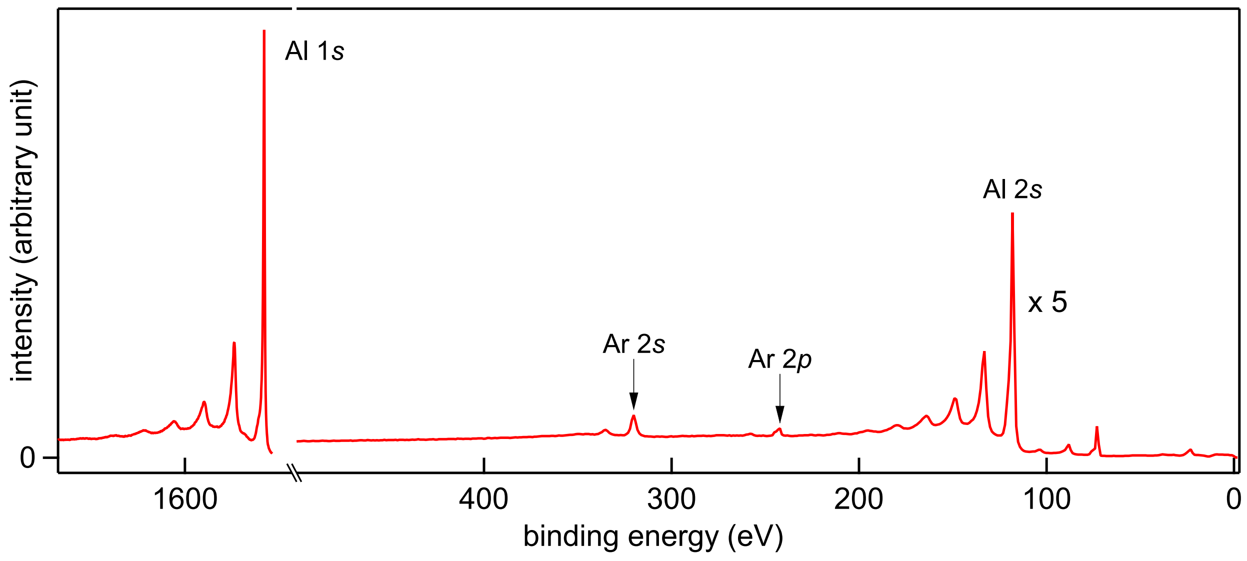


FIG. S 2. The survey spectrum of Al metal that shows the Al 1*s* and 2*s* main peaks and their loss regions. The region encompassing Al 2*s* from $E$= 500 eV to $E_F$ is depicted with a magnification of 5.

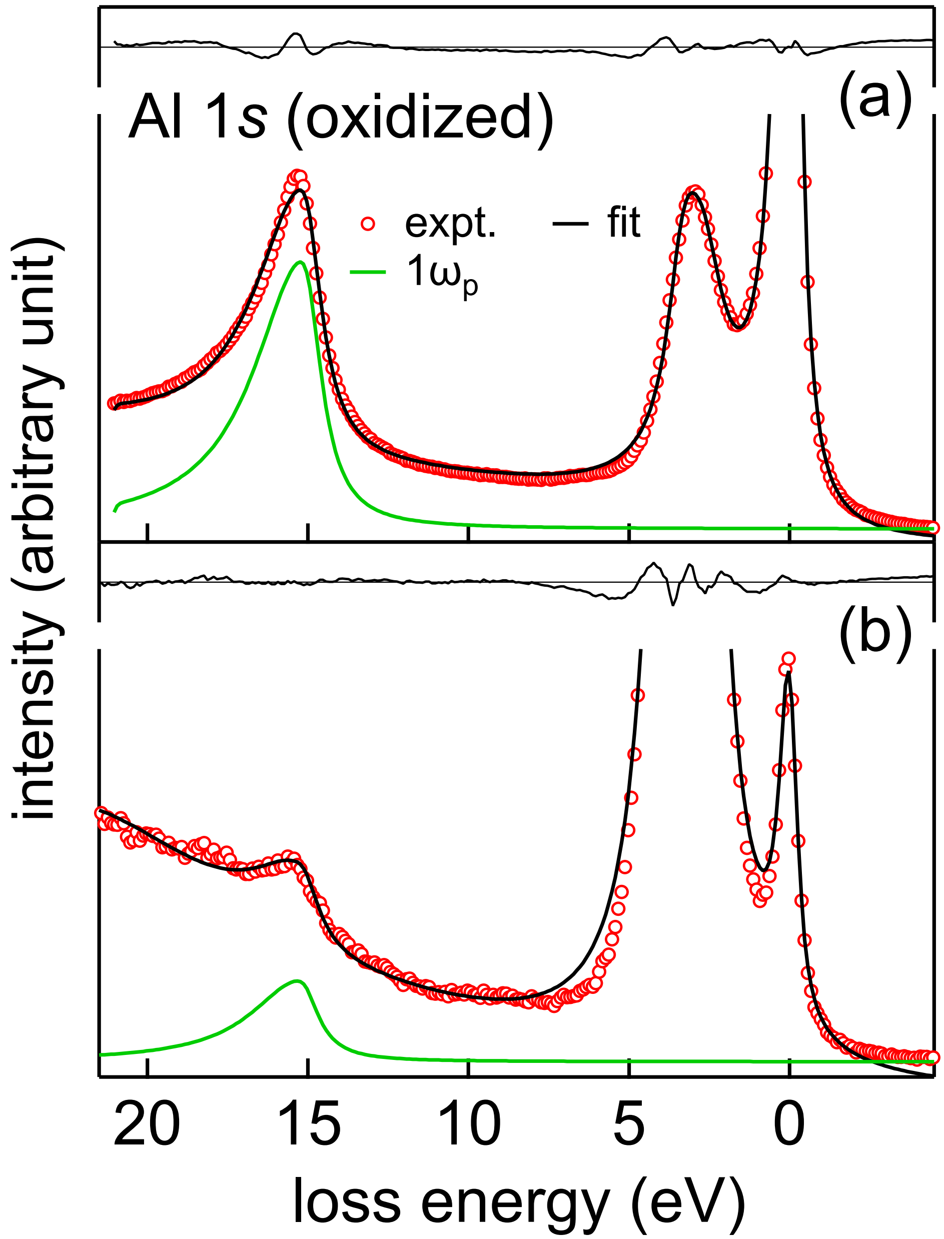


FIG. S 3. (a) Normal ($\theta$= 80°) and (b) grazing emission ($\theta$= 10°) Al 1$s$ core level spectra of fully oxidized Al surface. The fitted curve, $1\omega_p$, and the residual of fitting (top panel) are shown.

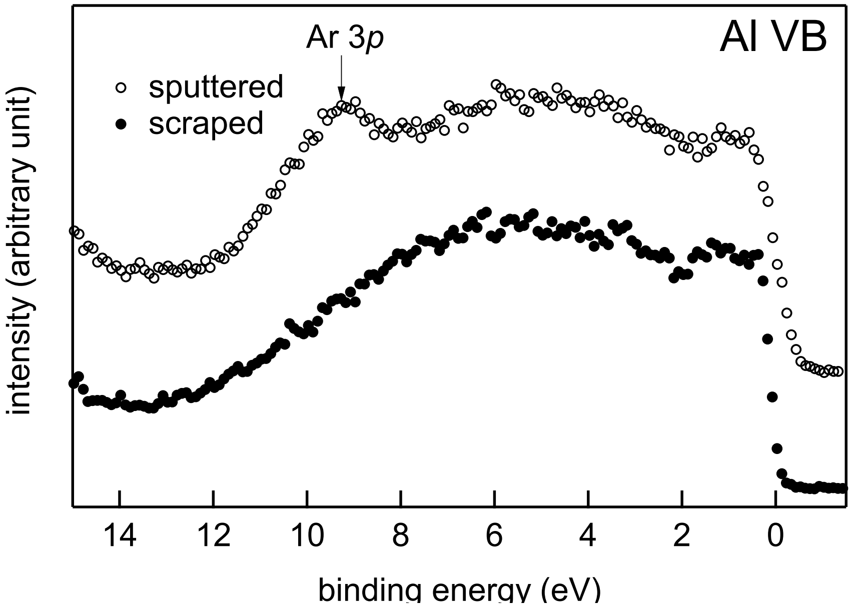


FIG. S 4. The HAXPES valence band (VB) of Al metal taken on a scraped surface and an $Ar^{+}$ ion sputtered surface. The Ar 3*p* peak in the latter is marked by an arrow.

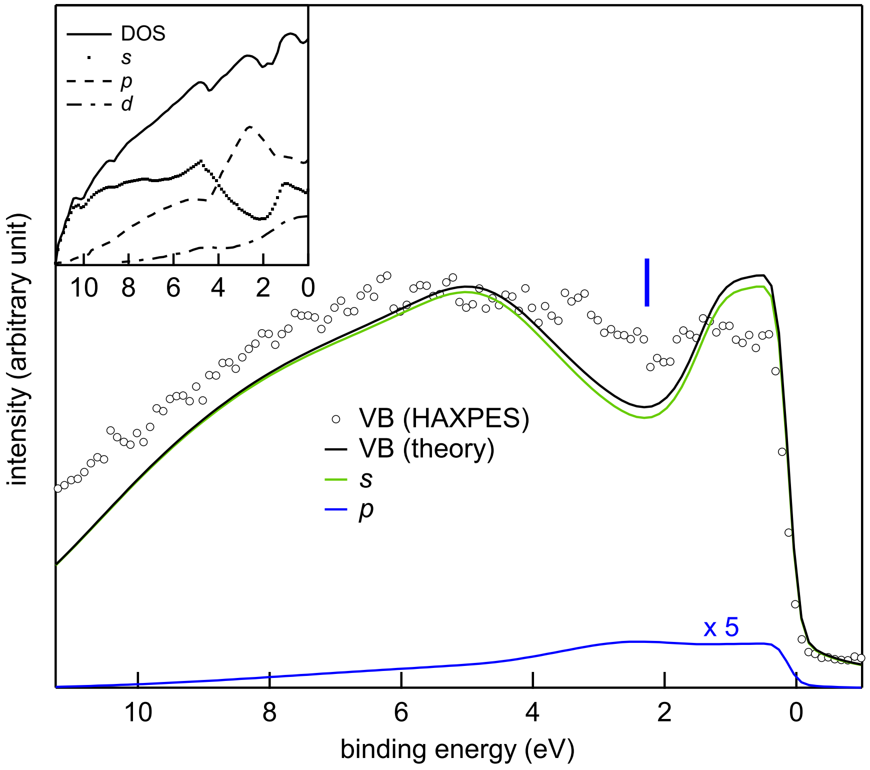


FIG. S 5. HAXPES VB of Al (open circles) compared with calculated VB (black curve) using the Al PDOS from the literature (see inset) calculated using the KKR method [4]. The *s* and *p* contributions are shown.

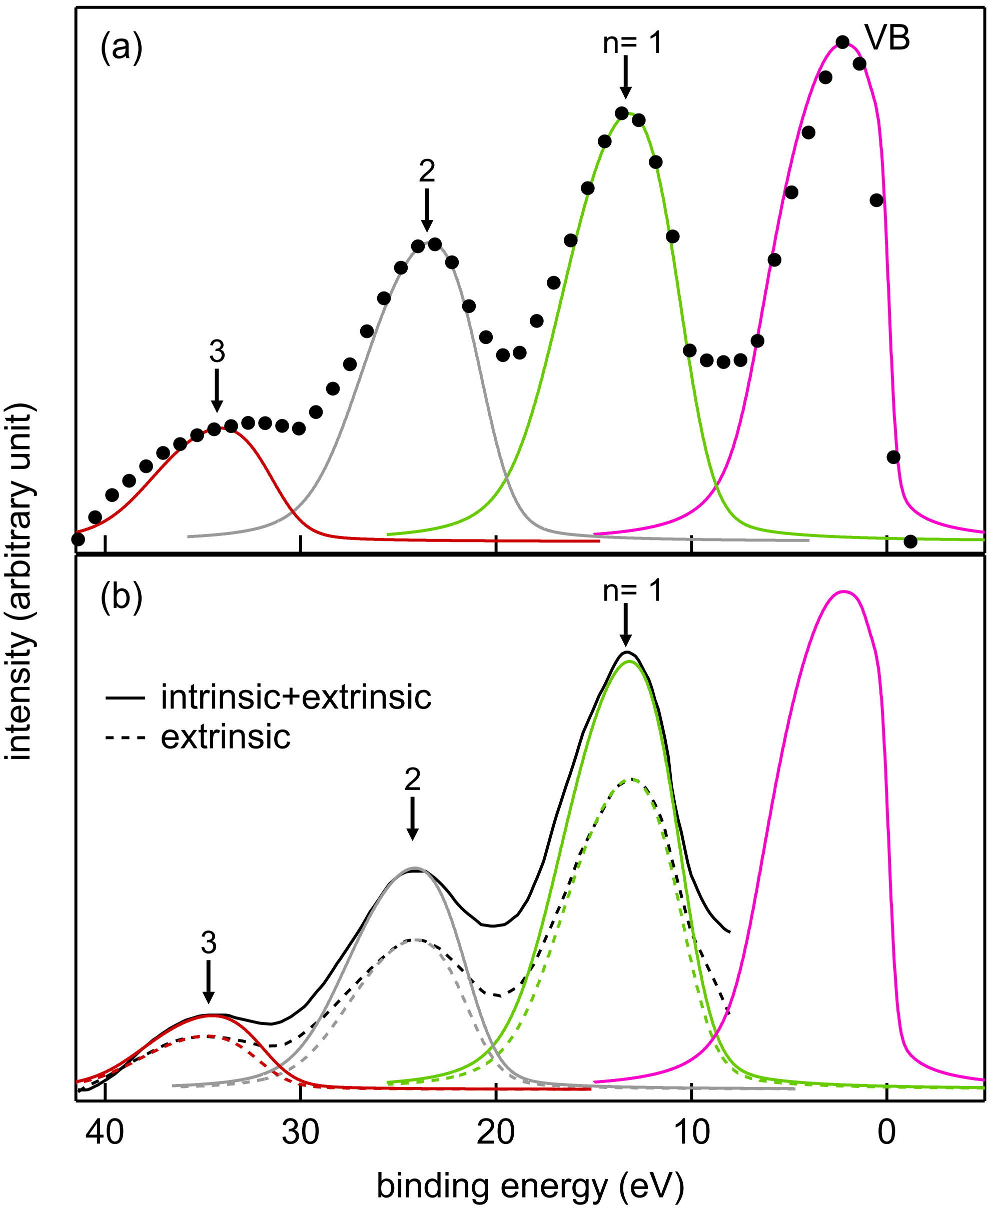


FIG. S 6. (a) VB XPS spectrum of Mg (black dots) from literature [2, 3] after inelastic background subtraction compared with calculated VB using PDOS in Fig. 5(g) (pink curve). The areas of VB plasmons marked as $n$= 1-3 are estimated by the green, gray, and red curves, respectively. (b) The VB plasmons from the literature [2] after inelastic background subtraction for $n$= 1-3 calculated with both intrinsic and extrinsic (solid black curve) and only extrinsic (dashed black curve) contributions. The areas of these plasmons have been estimated from the calculated XPS VB (pink curve) by shifting it by $n\omega_p$ and broadening, as shown by the green, gray, and red curves. The corresponding $b_{VB}(n)$ are plotted in Fig. 6 of the main manuscript.
